# Supplementary material for: Abstract Interpretation of Stateful Networks
Source: arXiv:1708.05904 source file (2018-07-04)
Supplement: Supplementary file 1 [file evaluation-appendix.tex]

\section{Datalog Translation}

The next example illustrates how a simple network is translated to Datalog.

\begin{figure}
\begin{center}
{\small
\begin{alltt}
// State initialization
abstract_state_sfw(this,h,false,false,false) <-
  host(h),            
  session_fw(this).
// Request packets from internal port
abstract_state_sfw(this,packet_dst,prev_0,prev_1,true) <-
  abstract_state_sfw(this,packet_dst,prev_0,prev_1,false),            
  portId[0]=int_port,
  typeId[0]=req_type,
  pending_no_src(this,packet_dst,req_type,int_port).
pending(mbox, src, dst, req_type, other_port) <-
  portId[1]=ext_port,
  link(this, ext_port, mbox, other_port),
  portId[0]=int_port,
  typeId[0]=req_type,
  pending(this,src,dst,req_type,int_port),
  session_fw(this).
// Communication from internal port
pending(mbox, src, dst, tp, other_port) <-
  portId[1]=ext_port,
  link(this, ext_port, mbox, other_port),
  portId[0]=int_port,
  pending(this,src,dst,tp,int_port),
  abstract_state_sfw_q0(this,dst,true),
  session_fw(this).
// Communication from external port
pending(mbox, src, dst, tp, other_port) <-
  portId[0]=int_port,
  link(this, int_port, mbox, other_port),
  portId[1]=ext_port,
  pending(this,src,dst,tp,ext_port),
  abstract_state_sfw_q1(this,src,true),
  session_fw(this).
// Response from external port
abstract_state_sfw(this,src,true,true,true) <-
  abstract_state_sfw_q2(this,src,true),            
  portId[1]=ext_port,
  typeId[1]=resp_type,
  pending_no_dst(this,src,resp_type,ext_port).

\end{alltt}
}
\end{center}
\caption{\label{fig:session-fw-datalog}%
An AMDL definition for the session firewall middlebox.}
\end{figure}

% \begin{tabbing}
% sf\=irewall= do \+ \\
% in\=t_pr ? p => \+ // internal port\\
% if\= \+\\
% p.dst in trusted => ext_pr ! p \(\Box\) \\
% p.\=type = 0 => // request packet \+ \\
% ext_pr ! p; \\
% requested(p.dst) := true \-\-\\
% fi \-\\
% ex\=t_pr ? p => \+ // external port\\
% if\= \+ \\
% p.src in trusted => int_pr ! p \(\Box\)\\
% p.\=type = 1 and p.src in requested => \+\\
% // response packet with a request\\
% trusted(p.src) := true \- \- \\
% fi \-\- \\
% od
% \end{tabbing}
% \end{alltt}
% }
% \end{center}
% \caption{\label{fig:session-fw-code}%
% An AMDL definition for the session firewall middlebox.}
% \end{figure}

\begin{example}
\TODO{Maybe show some of the LogicBlox code for the running example --- \Cref{fig:running-ex-topo}.}
\end{example}

\section{Further Evaluation}
